# Supplementary material for: Numerical Fuzz: A Type System for Rounding Error Analysis
Source: arXiv:2405.04612 source file (2025-04-08)
Supplement: Supplementary file 1 [file Appendix.tex]

\section{Appendix 1}\label{sec:app1}
